# Supplementary material for: The MAPS Algorithm: Fast model-agnostic and distribution-free prediction intervals for supervised learning
Source: arXiv:2410.08958 source file (2026-02-20)
Supplement: Supplementary file 1 [file classical_setup.tex]

\subsection{Additive errors and pivotal quantities} 
\label{subsec: additive errors}
The additive errors framework exploits~\eqref{eq: regression error} by assuming that data are generated by
\begin{equation} \label{eq: additive errors}
    Y = f (\boldsymbol{x}) + \epsilon,
\end{equation}
where $\epsilon \sim P_{\epsilon}$ are zero-mean, $\mathrm{var} (\epsilon) = \sigma_{\epsilon}^2 < +\infty$, and $f$ has a finite $L_2$-norm, i.e., $\int f^2 (\boldsymbol{x}) d P_{\bx} < +\infty$, $P_{\bx}$ is an unspecified distribution for the predictors, e.g., uniform over an unknown manifold, and the errors are independent of $\boldsymbol{X}$. In this case, the training and out-of-sample data are iid realisations coming from~\eqref{eq: additive errors}, where the error distribution does not depend on $f (\boldsymbol{x})$. We say that these are {\em homoscedastic} errors. Prediction intervals can be derived by obtaining pivotal quantities as done by~\cite{pivot}. We assume that the parametric family the error distribution belongs to is known (e.g., a zero-mean normal distribution with unknown variance), select a fitting procedure and specify a regression family, and use analytical methods for obtaining a known sampling distribution for the prediction error. For example, if we assume that the data are generated by the simple linear regression $Y = \beta_0 + \beta_1 x + \epsilon$, where $\epsilon \sim \mathcal{N} (0, \sigma_{\epsilon}^2)$, and estimate the unknown parameters by least-squares, i.e., $\hat{f}_{\ell r} (x_o) = \hat{\beta}_0 + \hat{\beta}_1 \, x_o$. Then, for $\hat{\sigma}_{\epsilon}^2 = 1 / (\ntrain - 2) \, \sum_{i = 1}^{\ntrain}  ( y_i -  \hat{f}_{\ell r} (x_i) )^2$ and $\hat{\epsilon}_o = Y_o - \hat{f}_{\ell r} (x_o)$ we have that
\begin{equation} \label{eq: classic prediction interval}
    \hat{\epsilon}_o \, \left \{ (\ntrain - 2) \, \hat{\sigma}_{\epsilon}^2 \ \left ( 1 + \frac{1}{ n_{\mathrm{train}} } + \frac{(x_o - \overline{x}_{\mathrm{train}})^2 }{ \sum_{i = 1}^{n_{\mathrm{train}}} (x_i - \overline{x}_{\ntrain})^2  } \right) \right \}^{ - 1 / 2}
    \sim t (\ntrain - 2),
\end{equation}
where $t(\ntrain -2)$ is Student's $t$-distribution with $(\ntrain - 2)$ degrees of freedom; see, e.g.,~\cite{linear_models_book}.
%, i.e., the training set mean-squared prediction error 
The standardised prediction error, i.e., the left-hand side in~\eqref{eq: classic prediction interval} is an important and well-known pivotal quantity (its distribution does not depend on unknown parameters). The prediction intervals $ \widehat{C}_{\ell r} (x_o) $ are
\begin{equation} \label{eq: classic lin reg interval}
     \hat{f}_{\ell r} (x_o) \pm \left \{ (\ntrain - 2) \, \hat{\sigma}_{\epsilon}^2 \ \left ( 1 + \frac{1}{ n_{\mathrm{train}} } + \frac{(x_o - \overline{x}_{\mathrm{train}})^2 }{ \sum_{i = 1}^{n_{\mathrm{train}}} (x_i - \overline{x}_{\ntrain})^2  } \right) \right \}^{1 / 2} t_{ (\ntrain - 2), 1 - \alpha / 2} ,
\end{equation}
where $t_{ (\ntrain - 2), \, 1 - \alpha / 2} $ is the $(1 - \alpha / 2)$-quantile of $t (\ntrain -2)$. If these modelling assumptions are valid, then the interval in \eqref{eq: classic lin reg interval} is a confidence interval for $y_o$ at the $(1 - \alpha) \times 100\%$, i.e., for all $x_o$ it has valid conditional coverage,
$\prob (  Y_o \in \widehat{C}_{\ell r} (x_o) \, | \, X_o = x_o ) = 1 - \alpha . $
\par
Note that $\hat{f}_{\ell r} (x_o)$ is a consistent estimator of $\beta_0 + \beta_1 x_o$, and since Student's $t$-distribution converges to a standard normal as $n_{\mathrm{train}} \to +\infty$. In view of Lemma~\ref{lem: oracle and ideal coverage}, we see that $\widehat{C}_{\ell r} (x_o)$ is longer and converges in probability to the ideal interval for simple linear regression,
\begin{equation*}
    (\beta_0 + \beta_1 \, x_o ) \pm \sigma_{\epsilon} \, z_{1 - \alpha / 2},
\end{equation*}
where $z_{1 - \alpha / 2}$ is the $(1 - \alpha/ 2)$-quantile of the standard normal distribution, note that $ | z_{1 - \alpha / 2} | <  | t_{ (\ntrain - 2), \, 1 - \alpha / 2} |$. We remark that deriving closed-form prediction intervals without imposing assumptions on $f$ and $P_{\epsilon}$ can be challenging. Alternatively, we can use computational techniques, e.g., cross-validation~\citep{stone_cv} for estimating the generalisation error and its distribution. Simply put, to compute a valid model-agnostic prediction interval, we must estimate the prediction residual distribution.
%length of the interval depends on how much the out-of-sample observation deviates from the training set mean, i.e., $(x_o - \overline{x}_{\mathrm{train}})^2$. Further, more accurate predictions produce tighter prediction intervals (smaller $\hat{\sigma}_{\epsilon}^2$). 
%Our objective is estimating the distribution of $\hat{\epsilon}$ for any model $\hat{f}$, i.e., we do not assume anything about $f$. 

%We enlist three settings for computing prediction intervals by increasing complexity below.
%\begin{itemize}
%    \item Perhaps the most stringent setting is the classic one, i.e., $\epsilon \sim \mathcal{N}(0, \sigma_{\epsilon}^2)$. This setting can be extended to other known error distributions, e.g., $\epsilon \sim \mathrm{Laplace} (0, b)$. We refer to it as homoscedastic additive errors with known distribution. 
%    \item A useful relaxation is working with heteroscedastic additive errors, i.e., the error variance depends on $\boldsymbol{x}$, but the error distribution is specified, e.g., $\epsilon \sim \mathcal{N}(0, \sigma_{\epsilon}^2 (\boldsymbol{x}))$. We refer to it as heteroscedastic additive errors with known distribution. 
%    \item Estimating the prediction error distribution with nonparametric methods, i.e., $P_{\epsilon}$ is not specified. We refer to it as nonparametric additive errors, which can be homoscedastic or heterosdastic.
%\end{itemize}
%We propose prediction intervals for each of these in Sections~\ref{sec: lpm} and~\ref{sec: maps}.
