# Supplementary material for: The MAPS Algorithm: Fast model-agnostic and distribution-free prediction intervals for supervised learning
Source: arXiv:2410.08958 source file (2026-02-20)
Supplement: Supplementary file 2 [file theorem_one_proof.tex]

\subsection{LPM with noise in the classic setting}
In the classic setting we assume that the LPM is given by
\begin{equation} \label{eq: classic setting lpm}
    \calb{Y} = y_{\beta} (\calb{\bx}) + u, 
\end{equation}
where $y_{\beta} (\calb{\bx}) := \beta_0 + \beta_1 \hat{f} (\calb{\bx})$, 
%$\var ( \calb{Y} ) = \var(f) + \sigma_{\epsilon}^2$, $\var(f) = \int \{f(\bx) - \mu(f) \}^2 dP_{\bx}$, $\mu(f) := \int f(\bx) dP_{\bx}$,
and the error linked to $\hat{f}$ is Gaussian, i.e., $u \sim \mathcal{N} (0, \sigma_{u}^2)$; see~\cite{salnikov2024liftedcoefficientdeterminationfast} for an earlier version of~\eqref{eq: classic setting lpm}. 
% \begin{remark}
    % The {\em LPM} given by~\eqref{eq: classic setting lpm} can be derived from a bivariate Gaussian assumption that links the correlation between calibration observations and model predictions;
%     Formally, it is derived from the conditional mean of $\calb{Y} \, | \, \hat{f} (\calb{\bx})$ if we assume that
%     \begin{equation*}
%     \begin{Bmatrix} 
%     \calb{Y} \\ \hat{f} (\calb{\bx}) 
%     \end{Bmatrix} \sim \mathcal{N}_2 \bigg [ \begin{Bmatrix} f(\calb{\bx}) \\ \overline{f} (\calb{\bx}) \end{Bmatrix},
%     \begin{pmatrix} \mathrm{var} (\calb{Y}) & \mathrm{cov} \{ \calb{Y}, \overline{f} (\calb{\bx}) \} \\ \mathrm{cov} \{ \calb{Y}, \overline{f} (\calb{\bx}) \} & \mathrm{var} (\overline{f}) \end{pmatrix} \bigg ].
% \end{equation*}
% \end{remark}
Note that~\eqref{eq: classic setting lpm} connects data generated by~\eqref{eq: regression error} with model predictions $\hat{f} (\calb{\bx})$ via a known joint distribution function. We stress that the random errors in~\eqref{eq: classic setting lpm} are {\em different} from the ones in~\eqref{eq: regression error}, i.e., $P_{u}$ is not the same as $P_{\epsilon}$, e.g., if~\eqref{eq: classic setting lpm} is valid, then $\var (u) = ( 1 - \rho^2) \{\var(f) + \sigma_{\epsilon}^2 \}$, which is equal to $\sigma_{\epsilon}^2$ if the regression function is constant, $f \equiv C$, or if $\beta_0 = 0$, $\beta_1 = 1$ and $\hat{f} \equiv f$ (in probability). Hence, we can derive a known prediction error distribution within the classic setting of linear regression with Gaussian errors. We estimate the unknown bias, $\beta_0$, and precision, $\beta_1$, coefficients in~\eqref{eq: classic setting lpm} by least-squares, and express the estimators in an alternative form, which highlights the interval's dependence on the correlation between model predictions and calibration response values.
The prediction interval, $\widehat{C}_{\ell pm} (\bx_o)$, is 
\begin{equation} \label{eq: b0 lpm prediction interval}
     \hat{y}_{\beta} (\bx_o) \pm \left \{ \left [1 + 1 / (n_{\mathrm{cal}} - 2) \right ] \left [ 1 - \calb{R^2} (\hat{f}) \right ] s_{\calb{\boldsymbol{y}}}^2 \left [ 1 + \widehat{\eta}_{\hat{f}} ( \boldsymbol{x}_o ) \right ] \right \}^{ 1 / 2 } t_{(n_{\mathrm{cal}} - 2), 1 - \alpha / 2},
\end{equation}
where $\hat{y}_{\beta} (\bx_o) := \hat{\beta}_0 + \hat{\beta}_1 \, \hat{f} (\x_o )$ are lifted predictions, $ \overline{\mu}_{\hat{f}} := ( 1 / \calb{n}) \, \sum_{\calb{i} = 1}^{\calb{n}} \hat{f} (\bx_{\calb{i}})$,
$$\widehat{\eta}_{\hat{f}} ( \boldsymbol{x}_o ) := \frac{1}{ n_{\mathrm{cal}} } + \frac{( \hat{f} (\bx_o) - \overline{\mu}_{\hat{f}})^2 }{ \sum_{i = 1}^{n_{\mathrm{cal}}} ( \hat{f} ( \bx_{\calb{i}}) -  \overline{\mu}_{\hat{f}})^2  }, $$
%% \begin{align*}
%     &\overline{y}_{\mathrm{cal}} = 1 / n_{\mathrm{cal}}  \sum_{i_{\mathrm{cal}} = 1}^{n_{\mathrm{cal}}} y_{i_{\mathrm{cal}}}, \, \, \, \, \, \, \, \, \, \, \, \,  s_{y_{\mathrm{cal}}}^2 = (n_{\mathrm{cal}} - 1)^{-1}  \sum_{i_{\mathrm{cal}} = 1}^{n_{\mathrm{cal}}} (y_{i_{\mathrm{cal}}} - \overline{y}_{\mathrm{cal}} )^2, \\
%     &\hat{\mu}_{\mathrm{cal}} = 1 / n_{\mathrm{cal}}  \sum_{i_{\mathrm{cal}} = 1}^{n_{\mathrm{cal}}} \hat{f} (\boldsymbol{x}_{i_{\mathrm{cal}}}), \, \, \, \, \, \,
%     s_{\hat{f}}^2 = (n_{\mathrm{cal}} - 1)^{-1}  \sum_{i_{\mathrm{cal}} = 1}^{n_{\mathrm{cal}}} \{ \hat{f} (\boldsymbol{x}_{i_{\mathrm{cal}}}) - \hat{\mu}_{\mathrm{cal}} \}^2,
% \end{align*}
% are sample mean and standard deviation statistics for response and model predictions in the calibration set, and
and $\calb{R} (\hat{f})$
    %$= \left [ \sum_{i_{\mathrm{cal}} = 1}^{n_{\mathrm{cal}}} (y_{i_{\mathrm{cal}}} - \overline{y}_{\mathrm{cal}})  \{ \hat{f} (\boldsymbol{x}_{i_{\mathrm{cal}}}) - \hat{\mu}_{\mathrm{cal}} \} \right ] / ( s_{y_{\mathrm{cal}}} \, s_{\hat{f}} )$
is the correlation coefficient between $\calb{\boldsymbol{y}}$ and $\{ \hat{f} (\boldsymbol{x}_{1_{\mathrm{cal}}}), \dots, \hat{f} (\boldsymbol{x}_{n_{\mathrm{cal}}}) \}$.
\par
The prediction interval $\widehat{C}_{\ell pm} (\bx_o)$ is model-agnostic at the $(1 - \alpha) \times 100\%$ confidence level, i.e., it is a valid non-trivial prediction interval for any model $\hat{f}$. Further, it suggests comparing predictive models using correlation values, since its length {\em decreases} the closer $R_{\mathrm{cal}}^2 (\hat{f})$ is to one, and that the MSPE of lifted predictions is smaller than the one of model predictions $\hat{f} (\calb{\bx})$.
%, i.e., $\sum_{\calb{i} = 1}^{\calb{n}} (y_{\calb{i}} - \hat{y}_{\beta} (\bx_{\calb{i}}) )^2 \leq \sum_{\calb{i} = 1}^{\calb{n}} (y_{\calb{i}} - \hat{f} (\bx_{\calb{i}}) )^2$. 
Theorem~\ref{th: t student interval} makes these statements precise.
\begin{theorem} \label{th: t student interval}
    Assume that~\eqref{eq: classic setting lpm} is valid. Then, given $\hat{f} (\boldsymbol{x}_o)$ and $\{ \hat{f} (\boldsymbol{x}_{1_{\mathrm{cal}}}), \dots, \hat{f} (\boldsymbol{x}_{n_{\mathrm{cal}}}) \}$, for all $\alpha \in (0, 1)$ we have that
    % \begin{equation} \label{eq: t-student distribution}
    %     U_o / \big \{ a^2 \big(1 - R^2_{\mathrm{cal}} (\hat{f}) \big) s_{y_{\mathrm{cal}}}^2 \hat{\eta} (\boldsymbol{x}_o ) \big \}^{ 1 / 2 } \sim t (n_{\mathrm{cal}} - 2),
    % \end{equation}
    % where $t (n_{\mathrm{cal}} - 2)$ is Student's t-distribution with $(n_{\mathrm{cal}} - 2)$ degrees of freedom. Thus, for $\alpha \in (0, 1)$ we have that
            \begin{equation} \label{eq: point estimator concentration}
                  \mathbf{Pr} \big ( Y_o \in \widehat{C}_{\ell pm} (\bx_o) \, | \, \bX_o = \bx_o \big ) = 1 - \alpha.
            \end{equation}
    Further, for homoscedastic errors, not necessarily Gaussian, the {\em MSPE} can be bounded as
    \begin{equation}
        \operatorname{MSPE} [ f (\bx_o)] \leq \operatorname{MSPE} [y_{\beta} (\bx_o)] \leq \operatorname{MSPE} [\hat{f} (\bx_o)],
    \end{equation}
    and we have that
    \begin{equation*}
        \operatorname{MSPE} [\hat{y}_{\beta} (\bx_o)] = \operatorname{MSPE} [y_{\beta} (\bx_o)] + o( 1 / \, \calb{n}).
    \end{equation*}
    % \begin{multline} \label{eq: mspe lower bound}
    %         \sigma_{\epsilon}^2 + \sigma_u^2 \mathbb{E} \big[ \widehat{\eta}_{\hat{f}} ( \boldsymbol{x}_o ) \big] \leq \operatorname{MSPE} [\hat{y}_{\beta} (\bx_o)]
    %         \leq \sigma_{\epsilon}^2 + \sigma_u^2 \mathbb{E} \big[ \widehat{\eta}_{\hat{f}} ( \boldsymbol{x}_o ) \big] \\
    %        + 2 \left ( \beta_1^2 \, \operatorname{MSPE} [\hat{f} (\bx_o)] + \{ \beta_0 + (\beta_1 - 1) f (\bx_o) \}^2 \right ).
    % \end{multline}
\end{theorem}
\par
Theorem~\ref{th: t student interval} allows us to compute fast model-agnostic conditional prediction intervals with valid finite sample coverage, albeit in the classic setting~\eqref{eq: classic setting lpm}. To the best of our knowledge, there are no other closed-form solution prediction intervals with these properties. Further, if $\hat{f}$ is consistent ($\| \hat{f} - f \|_{\infty} = o_{\mathbf{Pr}} (1)$), then $\hat{y}_{\beta}$ is also consistent, $| \hat{y}_{\beta} (\bx_o) - \hat{f} (\bx_o) | = o_{\mathbf{Pr}} (1)$ and $\widehat{C}_{\ell pm} (\bx_o)$ converges in probability to $C_{\mathrm{ideal}} (\bx_o)$. MAPS generalises $\widehat{C}_{\ell pm} (\bx_o)$ to the distribution-free setting.
